# Supplementary material for: One-stage Video Instance Segmentation: From Frame-in Frame-out to Clip-in Clip-out
Source: arXiv:2203.06421 source file (2022-03-12)
Supplement: Supplementary file 1 [file cis_sm.tex]

\begin{figure*}[!t]
\begin{center}
    \includegraphics[width=0.95\linewidth]{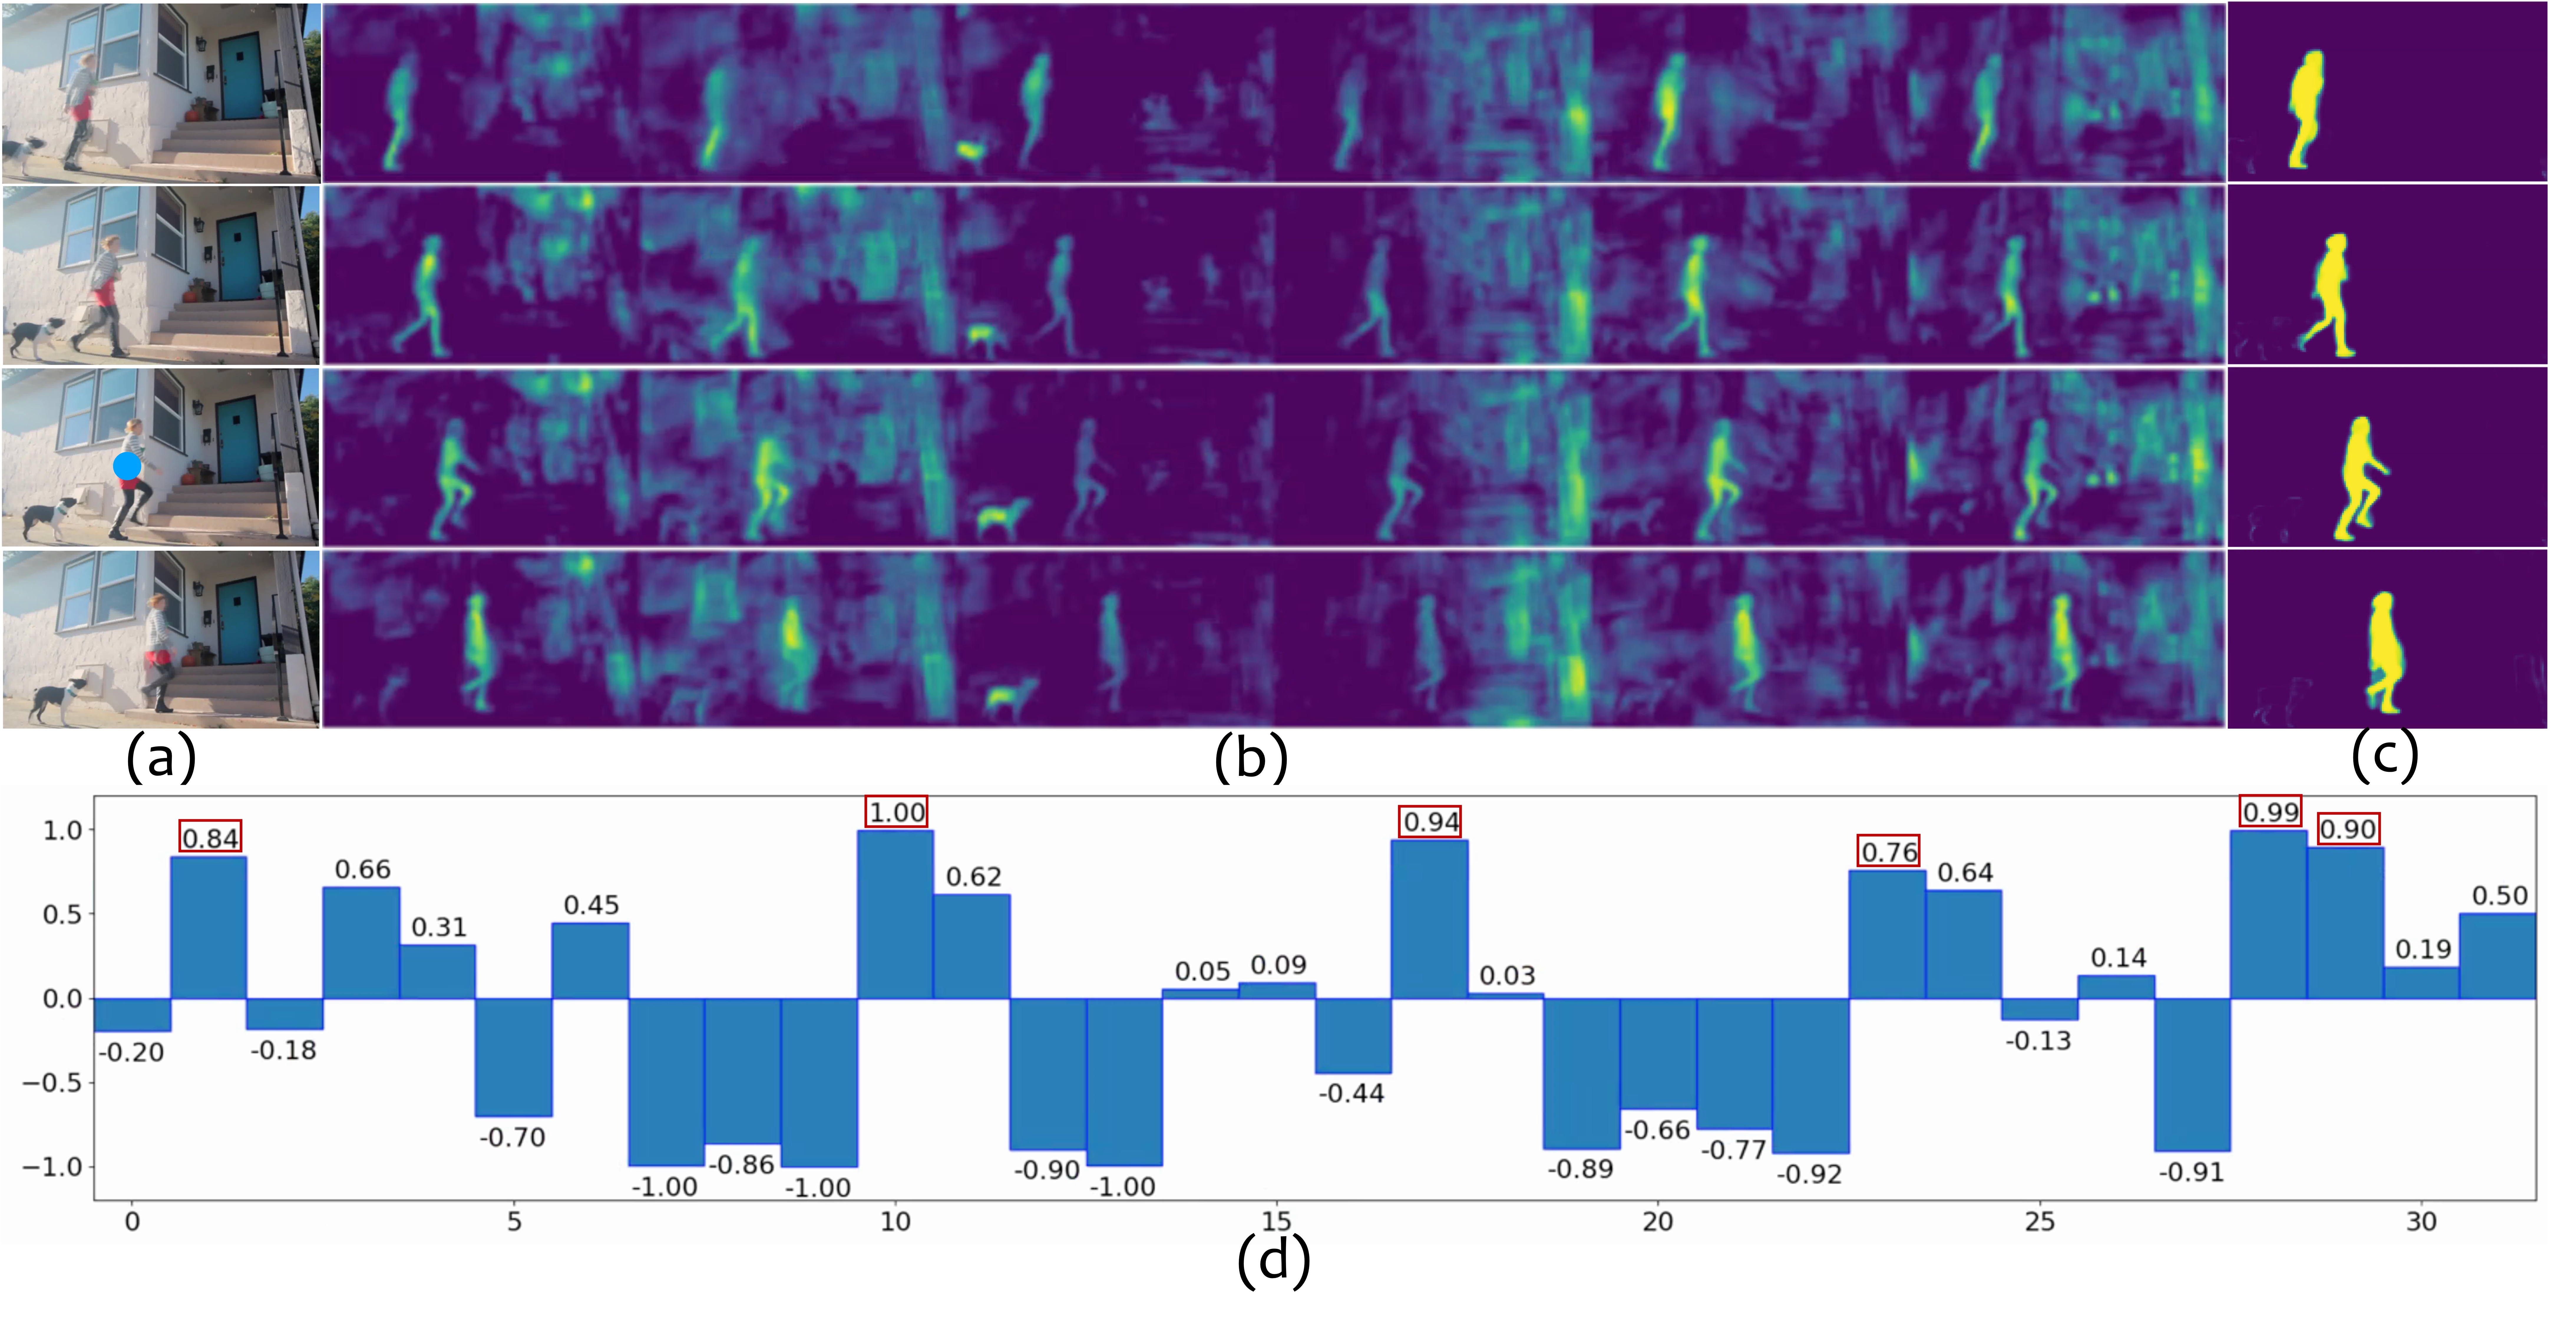}
\end{center}
\vspace{-9mm}
\caption{Illustration of the clip-level instance masks generation process of CiCo-Yolact by a video in YouTube-VIS 2019. (a) A 4-frame input clip; (b) a subset of clip-level prototypes (only the six prototypes whose corresponding coefficients are greater than 0.75 are shown here); (c) clip-level instance masks of an object; and (d) the shared 32-dim mask parameters of the object ($k\!=\!32$).  }\label{fig:cis_sm}
\vspace{-2mm}
\end{figure*}
